# Supplementary material for: Building an irreversible Carnot-like heat engine with an overdamped harmonic oscillator
Source: arXiv:2006.09426 ancillary file (2020-06-16)
Supplement: Supplementary file 1 [file sup_mat_v3_arxiv.pdf]

# Supplementary Material for "Building an irreversible Carnot-like heat engine with an overdamped harmonic oscillator"

**Carlos A. Plata**

Dipartimento di Fisica e Astronomia "Galileo Galilei", INFN, Università di Padova, Via Marzolo 8, 35131 Padova, Italy

**David Guéry-Odelin**

Laboratoire Collisions, Agrégats, Réactivité, IRSAMC, Université de Toulouse, CNRS, UPS, Toulouse, France

**Emmanuel Trizac**

Université Paris-Saclay, CNRS, LPTMS, 91405, Orsay, France.

**A. Prados**

Física Teórica, Universidad de Sevilla, Apartado de Correos 1065, E-41080 Sevilla, Spain

We put forward in this Supplementary Material some technicalities that complement our paper, but which are not necessary to understand its main results. Specifically, we provide an asymptotic analysis of the quasi-static limit in section 1. A detailed numerical exploration of the power and the efficiency for the full range of parameters is presented in section 2. We maximise the power and study its corresponding efficiency in the limit $\nu \to 1$—over the parameters $c$ and $d$, for fixed $\chi$—in section 3. Finally, this maximum power is further optimised over $\chi$ in section 4.

## 1. Approaching the quasi-static limit

Here we study the limit $(c, d) \to (1, 1)$, for given compression ratio $\chi$ and temperature ratio $\nu$, which corresponds to the quasi-static limit. We consider that both $\chi$ and $\nu$, and also $\mathcal{W}_\infty$, $\Delta_1$, and $\Delta_2$ are of the order of unity. This last condition guarantees the rigour of the following analysis.

As pointed out in the main text, when $c$ and $d$ approach unity, the time duration of both the adiabatic and isothermal branches diverge. That divergence is transferred to the parameter $\sigma$. Therefore, equation (42) of the main text can be written as

$$\tilde{\eta} - \eta_{\mathrm{C}} = \frac{\widetilde{\mathcal{W}}_2 + \widetilde{\mathcal{W}}_1 \nu}{\widetilde{\mathcal{W}}_1} + O(\sigma^{-1}) = -\nu \frac{\ln \frac{c}{d}}{\ln \chi} + O(\sigma^{-1}), \tag{S1}$$

that is,

$$\begin{aligned}\tilde{\eta}-\eta_{\mathrm{C}} &= O(1-c)+O(d-1)+O(\sigma^{-1}) \\ &= O(\tilde{s}_{BC}^{-1})+O(\tilde{s}_{DA}^{-1})+O((\tilde{s}_{BC}+\tilde{s}_{DA})^{-1/2}) \\ &= O((\tilde{s}_{BC}+\tilde{s}_{DA})^{-1/2}). \end{aligned} \tag{S2}$$

Therefore, the deviation from the Carnot efficiency scales in the limit as the square root of the total time in the adiabatic branches. The price to achieve such a high efficiency is paid by reducing the delivered power: the denominator in equation (40) of the main text diverges. In fact, since both $\tilde{s}_{AB}$ and $\tilde{s}_{CD}$ are $O(\sigma)=O((\tilde{s}_{BC}+\tilde{s}_{DA})^{1/2})$,

$$\widetilde{\mathcal{P}}=O((\tilde{s}_{BC}+\tilde{s}_{DA}+(\tilde{s}_{BC}+\tilde{s}_{DA})^{1/2})^{-1})=O((\tilde{s}_{BC}+\tilde{s}_{DA})^{-1}). \tag{S3}$$

Remarkably, the power vanishes faster than the efficiency tends to the Carnot value.

## 2. Numerical analysis for power and efficiency

In this section, we report the values of delivered power $\widetilde{\mathcal{P}}$ and efficiency $\tilde{\eta}$ as a function of the parameters $c, d$ for 9 couples of values of $(\nu,\chi)\in\{0.25,0.5,0.75\}\times\{0.25,0.5,0.75\}$ in Figs. 1, 2 and 3. This numerical exploration completes the study presented in the main text, where only the case $(\nu,\chi)=(0.75,0.5)$ was reported.

Specifically, figure 1 correspond to $\nu=0.25$, figure 2 to $\nu=0.5$, and figure 3 to $\nu=0.75$. Although the "grid" of values of $\chi$ presented is limited, some general conclusions can be extracted. For fixed $\nu$ and $\chi$, the point $(\tilde{c},\tilde{d})$ at which the maximum power is achieved is not always on the Curzon-Ahlborn line. However, its closeness increases as $\nu$ increases (for fixed $\chi$) and $\chi$ decreases (for fixed $\nu$). Also, for fixed $\nu$, there appears an optimal value of $\chi$, an optimal panel in each left column, so to say. In this optimal panel, the maximum power is always reached at a point very close to the Curzon-Ahlborn line (dashed): $\chi=0.25$ for both $\nu=0.25$ and $\nu=0.5$, and $\chi=0.5$ for $\nu=0.75$.

## 3. Maximisation with respect to $c$ and $d$ for $\nu\to 1$

This section and the next one are devoted to the analysis of the optimisation of the power and the study of the associated efficiency at maximum power. These calculations are performed in the limit as $\nu\to 1$. We introduce the following ansatz for the scalings of $1-c$, $1-d$:

$$c=1-\eta_{\mathrm{C}}^2\gamma, \quad d=1+\eta_{\mathrm{C}}^2\delta, \tag{S4}$$

where we consider both $\gamma$ and $\delta$ of the order of unity. The explanation for these scalings relies on the following qualitative argument.

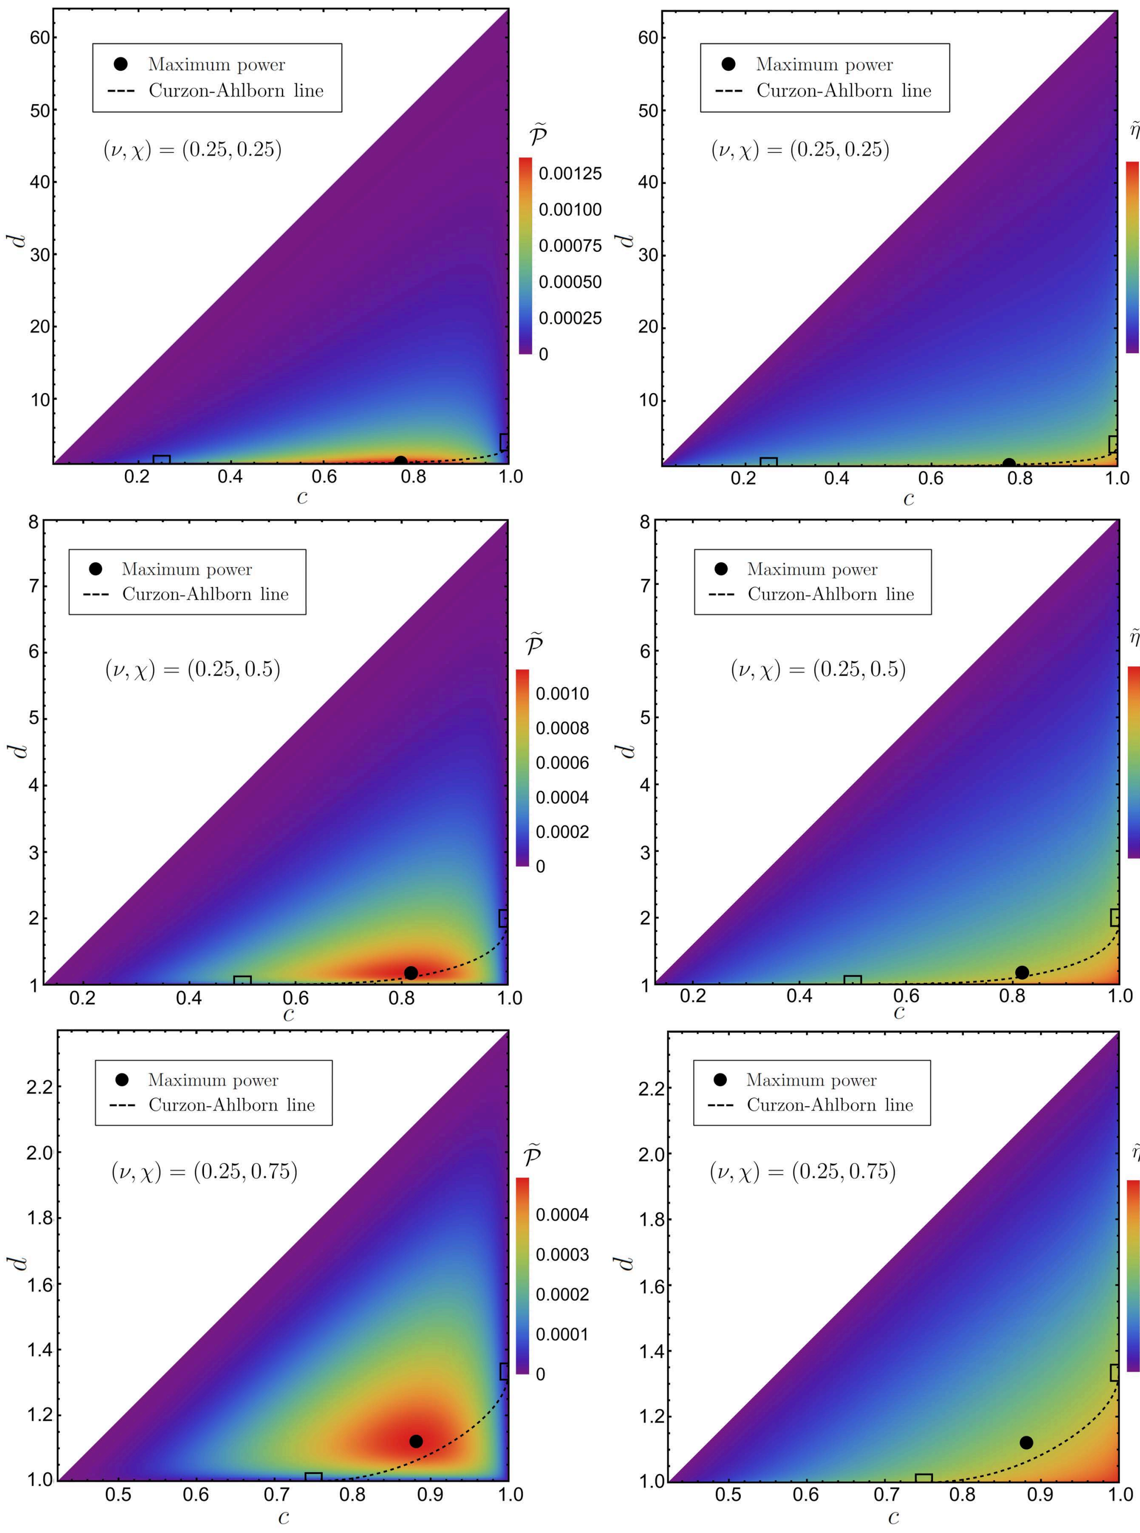


**Figure 1.** Density plots of the optimal power (left) and its corresponding efficiency (right) in the $(c, d)$ plane. The curves at which $\tilde{\eta} = \eta_{\rm CA}$ (dashed line), with its initial a final points (open squares) over the axes $d = 1$ and $c = 1$, respectively, and the point at which the maximum power (circle) is reached, are displayed in both panels. All graphs correspond to the same value of $\nu = 0.25$ and different values of $\chi = \{0.25, 0.5, 0.75\}$, from top to bottom.

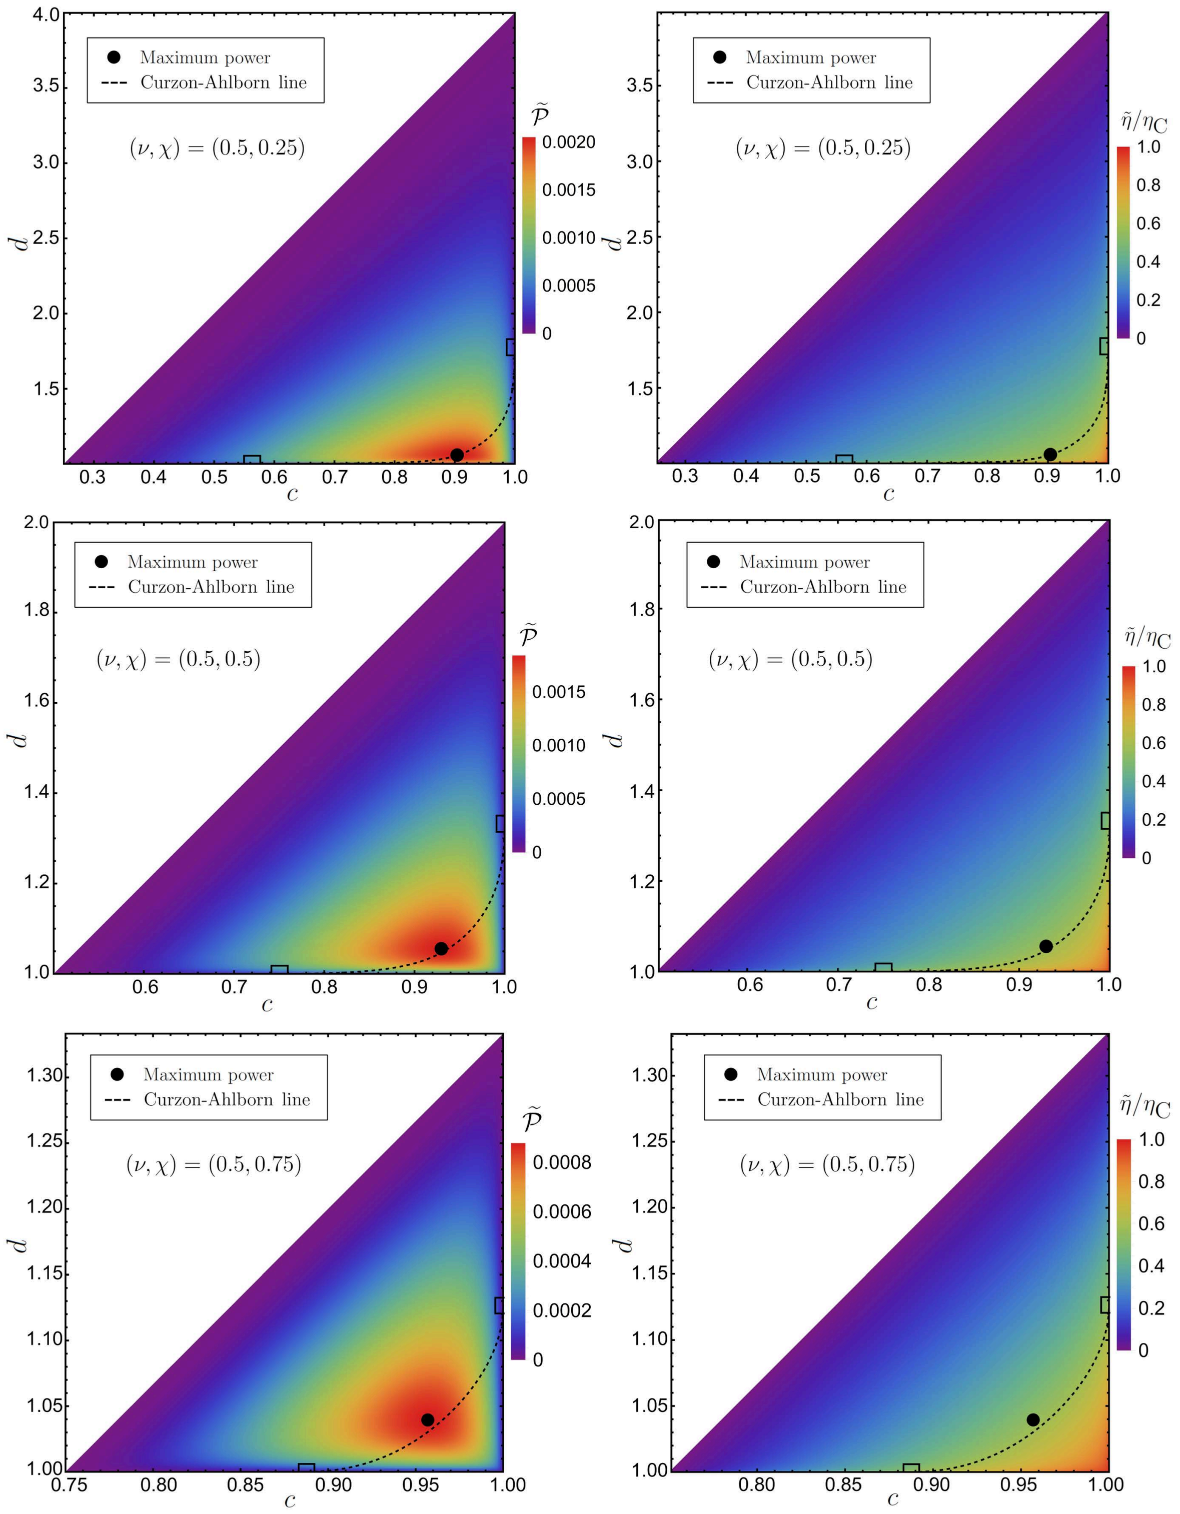


**Figure 2.** Same plots as in figure 1, but for $\nu = 0.5$.

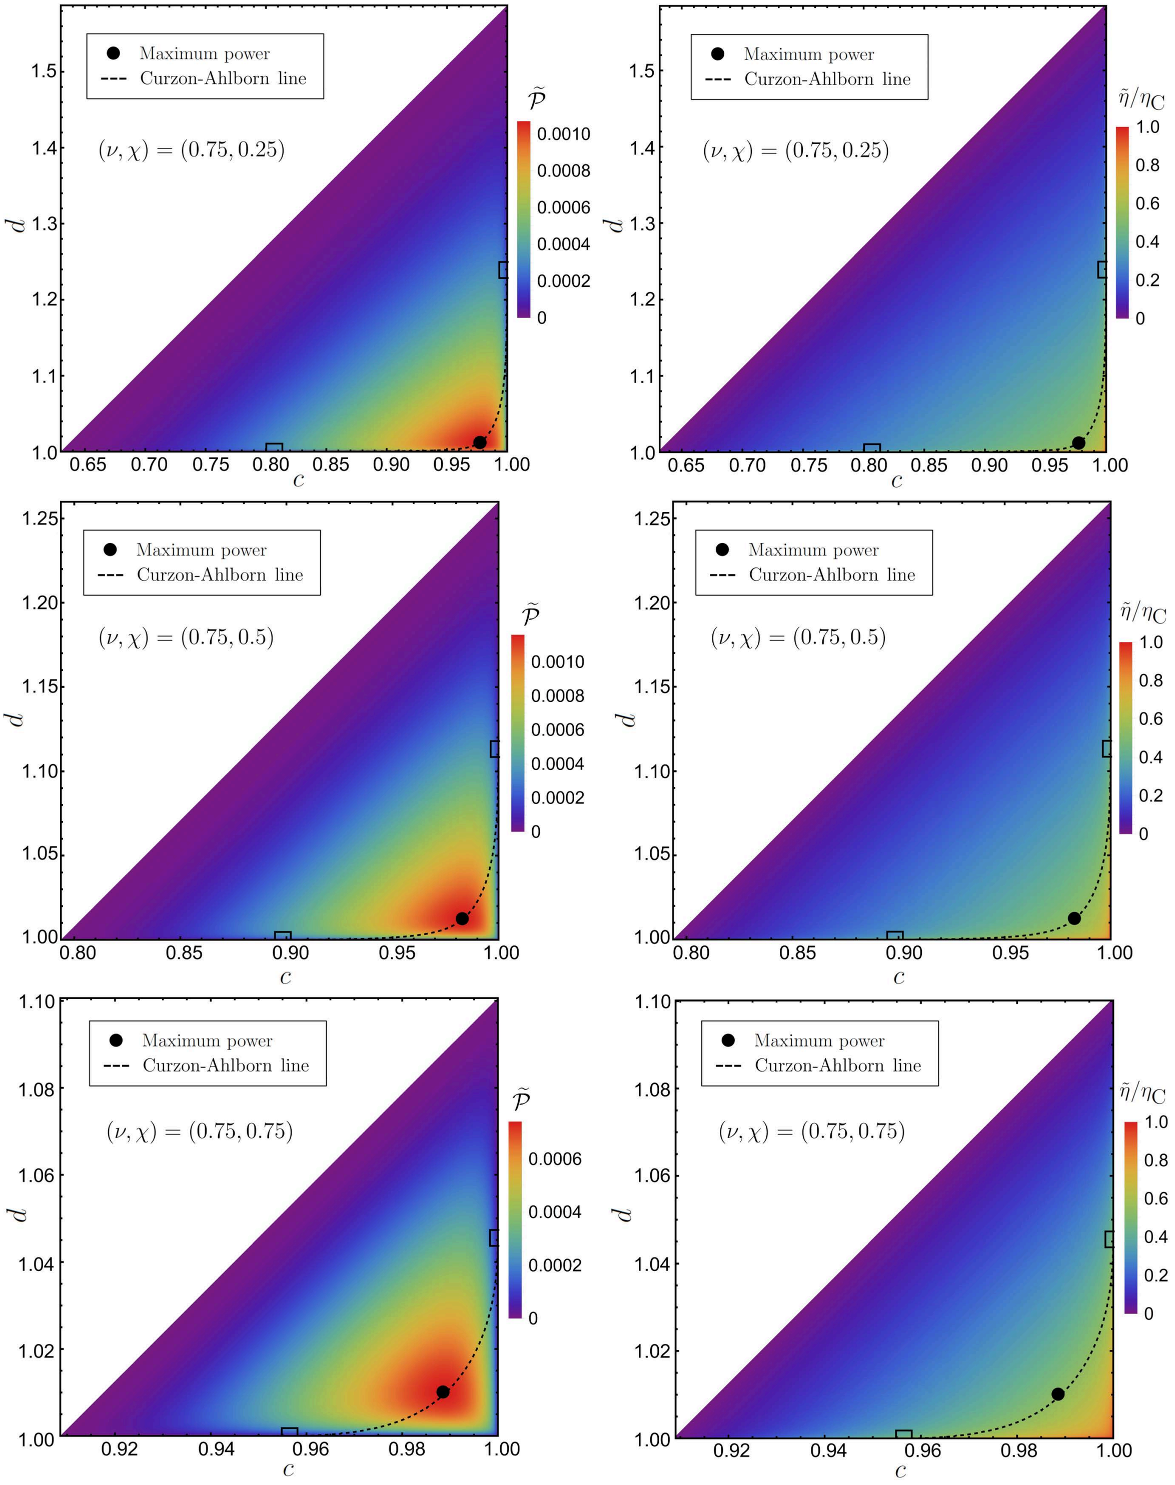


**Figure 3.** Same plots as in figure 1, but for $\nu = 0.75$. The central panels correspond to the ones reported in the main text.

*3.1. Justification for the scalings*

Let us start by looking at the total work for infinitely long in time isothermal processes $\mathcal{W}_\infty$ defined in equation (30) of the main text, which we can rewrite as

$$\mathcal{W}_\infty = \frac{1-\nu}{2}\ln\chi - \frac{\nu}{2}\ln\frac{c}{d} = \frac{\eta_\mathrm{C}}{2}\ln\chi - \frac{1-\eta_\mathrm{C}}{2}\ln\frac{c}{d}. \tag{S5}$$

Now, for a fixed value of $\chi$, of the order of unity, we consider that $\nu \to 1$ or $\eta_\mathrm{C} \ll 1$. In this regime, we would like to optimise our heat engine, in the sense we have been using throughout. Intuitively, we expect that the optimal values of $c$ and $d$ to be very close to 1. Then, we propose $c = 1 - \eta_\mathrm{C}^\alpha\gamma$, $d = 1 + \eta_\mathrm{C}^\beta\delta$, where $\gamma$ and $\delta$ are of the order of unity, and $\alpha, \beta > 0$ are to be determined by seeking a consistent limit, that is, a distinguished limit [1]. With these scalings,

$$\mathcal{W}_\infty \sim \frac{\eta_\mathrm{C}}{2}\ln\chi + \eta_\mathrm{C}^\alpha\frac{\gamma}{2} + \eta_\mathrm{C}^\beta\frac{\delta}{2}. \tag{S6}$$

We have to retain explicitly all the orders above because we do not know the specific values of $\alpha$ and $\beta$ yet.

Let us consider the asymptotic expansion of the optimal times over the adiabatic branches of the cycle. It is easy to show that

$$\tilde{s}_{BC} \sim \eta_\mathrm{C}^\alpha\frac{\gamma}{2\chi} + \eta_\mathrm{C}^{2-\alpha}\frac{1}{2\chi\gamma} + \eta_\mathrm{C}\frac{1}{\chi}, \quad \tilde{s}_{DA} \sim \eta_\mathrm{C}^\beta\frac{\delta}{2} + \eta_\mathrm{C}^{2-\beta}\frac{1}{2\delta} + \eta_\mathrm{C}. \tag{S7}$$

In order to have non-vanishing values of these optimal times, we have to impose that $\alpha = \beta = 2$. Next, we focus our attention on the optimal times over the isotherms. First, both $\Delta_1$ and $\Delta_2$ remain finite when $\eta_\mathrm{C} \to 0$ ($\nu \to 1$): by definition, $\Delta_1$ only depends on $\chi$ and

$$\Delta_2 \sim 1 - \frac{1}{\sqrt{\chi}} = -\Delta_1, \quad \Delta_1 - \Delta_2 \sim 2\Delta_1. \tag{S8}$$

We turn our attention to the parameter $\sigma$, defined in equation (35) of the main text. Since $\mathcal{W}_\infty \to 0$ and both $\tilde{s}_{BC}$ and $\tilde{s}_{DA}$ are of the order of unity, $\sigma$ is close to unity. Specifically,

$$\sigma - 1 \sim \eta_\mathrm{C}\frac{\left(\frac{1}{\chi\gamma} + \frac{1}{\delta}\right)\ln\chi}{32\Delta_1^2} \tag{S9}$$

where we have taken into account that

$$\tilde{s}_{BC} \sim \frac{1}{2\chi\gamma}, \qquad \tilde{s}_{DA} \sim \frac{1}{2\delta}, \quad \mathcal{W}_\infty \sim \underbrace{\frac{\eta_\mathrm{C}}{2}\ln\chi}_{\mathcal{W}_\infty^\mathrm{rev}} + \frac{\eta_\mathrm{C}^2}{2}\left(\gamma+\delta\right). \tag{S10}$$

The leading term in $\mathcal{W}_\infty$ coincides with the work in the reversible case, because the corrections introduced by $c$ and $d$ are of quadratic order.

Note that, with this scaling, the optimal times over the isotherms, as given by equation (36) of the main text, also diverge as $\eta_\mathrm{C}^{-1}$,

$$\tilde{s}_{AB} \sim \tilde{s}_\mathrm{iso}, \quad \tilde{s}_{CD} \sim \tilde{s}_\mathrm{iso}, \qquad \tilde{s}_\mathrm{iso} = \eta_\mathrm{C}^{-1}\frac{8\Delta_1^2}{-\ln\chi}. \tag{S11}$$

Therefore, the optimal times over the isotherms are much longer than those over the adiabatic parts of the cycle for fixed $\chi = O(1)$. This means that, when determining the optimal values $\tilde{c}$ and $\tilde{d}$, the leading behaviour is dominated by the isothermal branches.

With the obtained scaling, the leading term for the optimum power is

$$\widetilde{\mathcal{P}} \sim \frac{-\mathcal{W}_{\infty}^{\text{rev}}}{4\tilde{s}_{\text{iso}}} = \eta_{\text{C}}^2 \frac{(\ln\chi)^2}{64\Delta_1^2}, \tag{S12}$$

where we have taken into account that $\sigma \to 1$. With respect to the corresponding efficiency, $\tilde{\eta} \sim \mathcal{W}_{\infty}^{\text{rev}}/(2\mathcal{W}_1)$. Since $\mathcal{W}_{\infty}^{\text{rev}}$ and $\mathcal{W}_1$ are the total work and the work over the first isotherm in the reversible case, respectively, it is clear that

$$\tilde{\eta} \sim \frac{1}{2}\eta_{\text{C}} \tag{S13}$$

and we recover the "classical" linear response result.

### *3.2. Maximal power and associated efficiency*

Substituting the above proposed scalings into equation (40) of the main text, we find

$$\begin{aligned}\widetilde{\mathcal{P}} = {} & \eta_{\text{C}}^2 \frac{\chi(\ln\chi)^2}{64\left(1-\sqrt{\chi}\right)^2} \\ & + \eta_{\text{C}}^3 \frac{\chi\ln\chi\left\{16\gamma\delta\left(1-\sqrt{\chi}\right)^2\left[4(\gamma+\delta)-\ln\chi\right]+(\gamma\chi+\delta)(\ln\chi)^2\right\}}{2048\gamma\delta\left(1-\sqrt{\chi}\right)^4} \\ & + O(\eta_{\text{C}}^4)\end{aligned} \tag{S14}$$

for the power. On the other hand, the corresponding efficiency is

$$\tilde{\eta} = \frac{\eta_{\text{C}}}{2} + \eta_{\text{C}}^2\left[\frac{1}{8} + \frac{64\gamma\delta(\gamma+\delta)(1-\sqrt{\chi})^2-(\gamma\chi+\delta)(\ln\chi)^2}{128\gamma\delta(1-\sqrt{\chi})^2\ln\chi}\right] + O(\eta_{\text{C}}^3). \tag{S15}$$

The lowest order contributions in equations (S14) and (S15) have been obtained above, see equations (S12) and (S13), as a direct consequence of the scalings proposed in equation (S4).

Now, we enforce that $\partial\widetilde{\mathcal{P}}/\partial\gamma$ and $\partial\widetilde{\mathcal{P}}/\partial\delta$ vanish at the optimal values $\tilde{\gamma}$, $\tilde{\delta}$, which leads to the result

$$\tilde{\gamma} = \underbrace{-\frac{\ln\chi}{8(1-\sqrt{\chi})}}_{\tilde{\gamma}_0} + O(\eta_{\text{C}}), \qquad \tilde{\delta} = \underbrace{-\frac{\sqrt{\chi}\ln\chi}{8(1-\sqrt{\chi})}}_{\tilde{\delta}_0=\sqrt{\chi}\,\tilde{\gamma}_0} + O(\eta_{\text{C}}). \tag{S16}$$

Substitution of these values into equation (S14) gives

$$\widetilde{\mathcal{P}} = \underbrace{\eta_{\text{C}}^2 \frac{\chi(\ln\chi)^2}{64\left(1-\sqrt{\chi}\right)^2} - \eta_{\text{C}}^3 \frac{\chi(\ln\chi)^2}{64\left(1-\sqrt{\chi}\right)^3}}_{\widetilde{\mathcal{P}}_0} + O\left(\eta_{\text{C}}^4\right). \tag{S17}$$

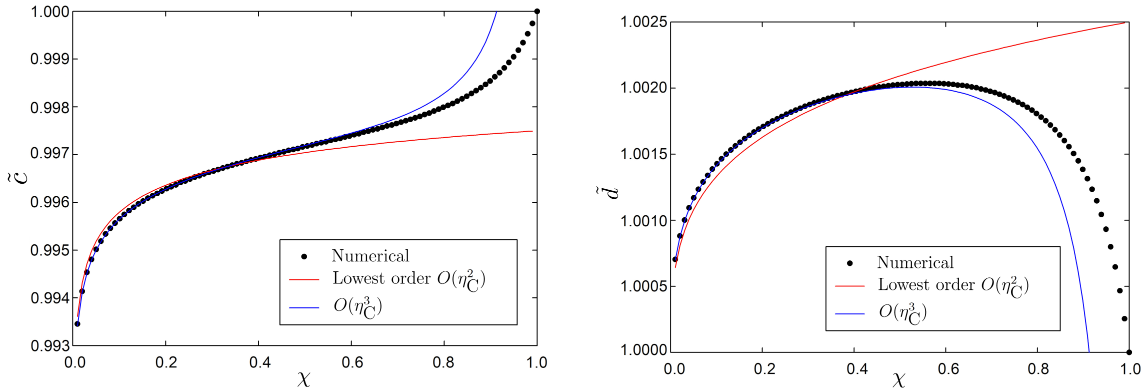


**Figure 4.** Optimal values $\tilde{c}$ and $\tilde{d}$ as a function of $\chi$ for $\nu = 0.9$ ($\eta_C = 0.1$). We compare the numerical results (circles) with the perturbative expansion in $\eta_C$ up to order $O(\eta_C^2)$ (red line) and up to order $O(\eta_C^3)$ (blue line).

for the optimal power. Note that we use the same symbol for the maximum power, $\widetilde{\mathcal{P}}$, but it depends only on $\nu$ and $\chi$ because it has been maximised with respect to $c$ and $d$. The efficiency at maximum power is then

$$\tilde{\eta} = \underbrace{\frac{\eta_C}{2} + \frac{\eta_C^2}{8}}_{\tilde{\eta}_0} + O(\eta_C^3), \tag{S18}$$

which coincides with the Curzon-Ahlborn limit up to the considered precision. Interestingly, this efficiency is "universal", in the sense that it is independent of the compression ratio $\chi$.

We can go to higher orders in the expansion of $\widetilde{\mathcal{P}}$ and $\tilde{\eta}$ in powers of $\eta_C$. We list the results without the (rather) lengthy derivations. The optimal values $\tilde{c}$ and $\tilde{d}$ are given by

$$\tilde{\gamma} = \tilde{\gamma}_0 + \eta_C\, \tilde{\gamma}_1 + O(\eta_C^2), \quad \tilde{\delta} = \tilde{\delta}_0 + \eta_C\, \tilde{\delta}_1 + O(\eta_C^2), \tag{S19}$$

where

$$\tilde{\gamma}_1 = \frac{\left(12\sqrt{\chi} - \ln\chi - 8\right)\ln\chi}{64\left(1-\sqrt{\chi}\right)^2}, \quad \tilde{\delta}_1 = \frac{\left(12\chi - \chi\ln\chi - 8\sqrt{\chi}\right)\ln\chi}{64\left(1-\sqrt{\chi}\right)^2}. \tag{S20}$$

In Figure 4, we compare the numerical solution of the optimal values $\tilde{c}$ and $\tilde{d}$ with our perturbative expansion in $\eta_C$. The agreement for values of $\chi$ not too close to unity is quite good. As $\chi \to 1$ the agreement worsens and the relative positions of the numerical and the theoretical curves change as higher order terms are introduced in the expansion in powers of $\eta_C$. This is a signature of the emergence of a quite wide boundary layer as $1-\chi$ goes to zero, inside which the current expansion in integer powers of $\eta_C$ breaks down. In fact, the width of this boundary layer is proportional to $\eta_C^{1/2}$ and a different approach is needed if one wants to further optimise the power with respect to $\chi$, see section 4 for further detail.

The efficiency at maximum power is now given by

$$\widetilde{\mathcal{P}} = \widetilde{\mathcal{P}}_0 + \eta_{\mathrm{C}}^4 \, \frac{\chi (\ln \chi)^2 \left(1 - \chi + 6\sqrt{\chi} + \ln \chi\right)}{512 \left(1 - \sqrt{\chi}\right)^4} + O\left(\eta_{\mathrm{C}}^5\right). \tag{S21}$$

The corresponding efficiency is

$$\tilde{\eta} = \tilde{\eta}_0 + \eta_{\mathrm{C}}^3 \, \frac{\chi - 1 - \ln \chi}{32 \left(1 - \sqrt{\chi}\right)^2} + O\left(\eta_{\mathrm{C}}^4\right). \tag{S22}$$

We observe that the $O(\eta_{\mathrm{C}}^3)$ is no longer universal and depends on the compression ratio $\chi$, thus deviating from the Curzon-Ahlborn bound. At order $O(\eta_{\mathrm{C}}^3)$, the deviation of the efficiency at optimal power from the Curzon-Ahlborn value has been previously reported in references [2, 3].

## 4. Maximisation with respect to $\chi$

In the previous section, the power has been optimised with respect to $(c, d)$ for fixed values of the temperature ratio $\nu$ and the compression ratio $\chi$. Here, we analyse the maximisation of this optimal power with respect to $\chi$, i.e. we seek the optimal value of the compression ratio $\tilde{\chi}$ for fixed $\nu$.

Let us have a closer look at the dependence of $\widetilde{\mathcal{P}}_0$ on $\chi$. On the one hand, the first term in $\widetilde{\mathcal{P}}_0$, $O(\eta_{\mathrm{C}}^2)$, is a monotonically increasing function of $\chi$. On the other hand, the second term in $\widetilde{\mathcal{P}}_0$, $O(\eta_{\mathrm{C}}^3)$, monotonically decreases. The combination of these two behaviours implies that $\widetilde{\mathcal{P}}_0$ has a maximum for a certain optimal value $\tilde{\chi}$. Moreover, since the second term in $\widetilde{\mathcal{P}}_0$ diverges as $\chi \to 1$, we expect $\tilde{\chi}$ to be close to unity, that is,

$$\tilde{\chi} = 1 - \eta_{\mathrm{C}}^x \, \Xi, \qquad \Xi = O(1) \tag{S23}$$

where $x > 0$ has to be determined by some *distinguished limit* argument.

### *4.1. Justification for the scaling*

We check our scaling ansatz (S23) by plotting the optimal power $\widetilde{\mathcal{P}}$ we looked at in the previous section, i.e. optimised with respect to $c$ and $d$, as a function of $\chi$. This is done for several values of $\eta_{\mathrm{C}}$ in figure 5, in which the optimal values $\tilde{c}$ and $\tilde{d}$ have been obtained numerically. It is neatly observed that $\widetilde{\mathcal{P}}$ (i) goes to 0 for $\chi \to 1$, (ii) has a maximum at a certain value $\tilde{\chi}$ (marked by a red triangle), with $\tilde{\chi} \to 1$ as $\eta_{\mathrm{C}} \to 0$.

Intuitively, one could think that, since $\tilde{\chi} \to 1$, the efficiency at optimal power can be obtained by taking the limit as $\chi \to 1$ of $\tilde{\eta}$ in equation (S22). In fact, this would lead to $\tilde{\eta} = \tilde{\eta}_0 + \eta_{\mathrm{C}}^3/16 + O\left(\eta_{\mathrm{C}}^4\right)$, which coincides with the Curzon-Ahlborn result to third order in $\eta_{\mathrm{C}}$. Notwithstanding, this is wrong. The reason is that some of the functions of $\chi$ that act as coefficients in the expansion in powers of $\eta_{\mathrm{C}}$ diverge as $\eta_{\mathrm{C}}^y$, with some $y < 0$, when the scaling (S23) is considered. Loosely speaking, this gives rise to a "renormalisation" of some of the previous coefficients in the expansion. See the following paragraphs for a thorough discussion of this issue and the correct value for the efficiency at maximum power.

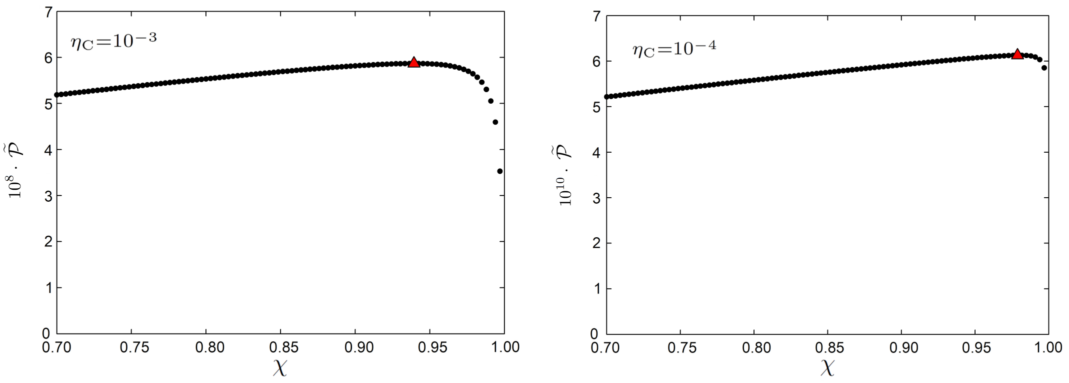


**Figure 5.** Maximum power as a function of $\chi$ for two different temperature ratios, $\eta_C = \{10^{-3}, 10^{-4}\}$. The maximum of each curve $(\tilde{\mathcal{P}}, \tilde{\chi})$ is marked by a red triangle, which approaches 1 as $\eta_C$ decreases.

Naively, one may try to obtain the value of $x$ in equation (S23) by arguing that the first and second terms in $\widetilde{\mathcal{P}}_0$ should be of the same order, which leads to $x = 1$. Notwithstanding, it can be shown that this scaling does not lead to a consistent prediction for $\tilde{\chi}$. The reason is that $\tilde{\chi}$ is determined by the vanishing of $\partial\widetilde{\mathcal{P}}/\partial\chi$, and therefore we have to impose the derivatives with respect to $\chi$ of the two terms in $\widetilde{\mathcal{P}}_0$ to be of the same order. Specifically, by taking into account that

$$\frac{\partial\widetilde{\mathcal{P}}_0}{\partial\chi} = \eta_C^2 \frac{\left[2(1-\sqrt{\chi}) + \ln\chi\right]\ln\chi}{\left(1-\sqrt{\chi}\right)^3} + \eta_C^3 \frac{\left[4(1-\sqrt{\chi}) + \left(\sqrt{\chi}+2\right)\ln\chi\right]\ln\chi}{2\left(1-\sqrt{\chi}\right)^4}, \tag{S24}$$

we can write

$$\frac{\partial\widetilde{\mathcal{P}}_0}{\partial\chi} \sim 2\eta_C^2 - 8\eta_C^3 \frac{1}{(1-\chi)^2}, \quad \chi \to 1^-. \tag{S25}$$

Thus, $x = 1/2$ to have comparable terms and, moreover, $\tilde{\Xi} \to 2$ as $\eta_C \to 0$.

In order to check the above scaling, we have numerically evaluated $\tilde{\chi}$ as a function of $\eta_C$ in the range $10^{-4} < \eta_C < 10^{-2}$. In figure 6, we plot $(1-\tilde{\chi})$ vs. $\eta_C$ in which we find a power-law behaviour with exponent very close to 1/2, in agreement with our theoretical prediction. In light of the above discussion, we finally propose the scaling

$$\chi = 1 - \eta_C^{1/2}\,\Xi, \quad \Xi = O(1), \quad \eta_C \ll 1. \tag{S26}$$

### *4.2. Maximal power and associated efficiency*

To get consistent expansions in powers of $\eta_C^{1/2}$ for a given $\nu$, we need to carry out the expansion after introducing all the scalings, for $(\chi, c, d)$, at the same time. In this way, we obtain

$$\widetilde{\mathcal{P}} = \frac{\eta_C^2}{16} - \eta_C^{5/2} \frac{(\gamma+\delta)(1+16\gamma\delta) + 4\gamma\delta\Xi^2}{128\gamma\delta\Xi} + O(\eta_C^3), \tag{S27}$$

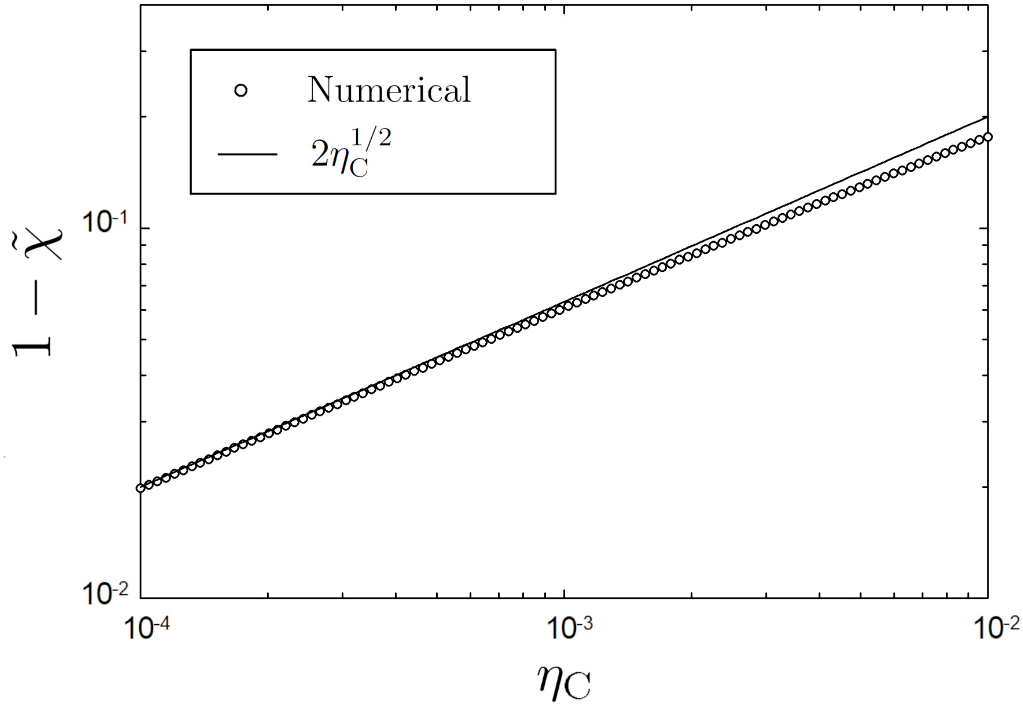


**Figure 6.** Optimal value for $\chi$ as a function of $\eta_C$. We choose to represent $1-\tilde{\chi}$ vs. $\eta_C$ in logarithmic scale in order to obtain the scaling exponent as the slope. This exponent is in quite good agreement with our theoretical prediction 1/2, especially for low values of $\eta_C$.

for the power, whereas we have

$$\tilde{\eta} = \frac{\eta_C}{2} - \eta_C^{3/2}\frac{(\gamma+\delta)(1-16\gamma\delta)}{32\gamma\delta\Xi} + O(\eta_C^2). \tag{S28}$$

for the efficiency.

Now, we want to seek the optimal values $(\tilde{\Xi}, \tilde{\gamma}, \tilde{\delta})$: thus, we enforce the vanishing of the partial derivatives of $\mathcal{P}$ with respect to $(\Xi, \gamma, \delta)$. This leads to

$$\tilde{\Xi} = 2 + O(\eta_C^{1/2}), \quad \tilde{\gamma} = \frac{1}{4} + O(\eta_C^{1/2}), \quad \tilde{\delta} = \frac{1}{4} + O(\eta_C^{1/2}). \tag{S29}$$

Note that the values of $\tilde{\gamma}$ and $\tilde{\delta}$ are the same that we could obtain by taking the limit $\chi \to 1$ in equation (S16). Up to this order we get that the maximum power for a given $\nu$ and its corresponding efficiency are

$$\widetilde{\mathcal{P}} = \frac{\eta_C^2}{16} - \frac{\eta_C^{5/2}}{8} + O(\eta_C^3), \quad \tilde{\eta} = \frac{\eta_C}{2} + O(\eta_C^2). \tag{S30}$$

We would like to obtain the efficiency at optimal power up to order $\eta_C^3$. Thus, we need $(\tilde{\Xi}, \tilde{\gamma}, \tilde{\delta})$ up to order $\eta_C^{3/2}$. To do so, we need to impose the vanishing of the partial derivatives up to order $\eta_C^4$, which gives the result

$$\tilde{\Xi} = 2 - \frac{8}{3}\eta_C^{1/2} + \frac{29}{9}\eta_C - \frac{2111}{540}\eta_C^{3/2} + O(\eta_C^2), \tag{S31}$$

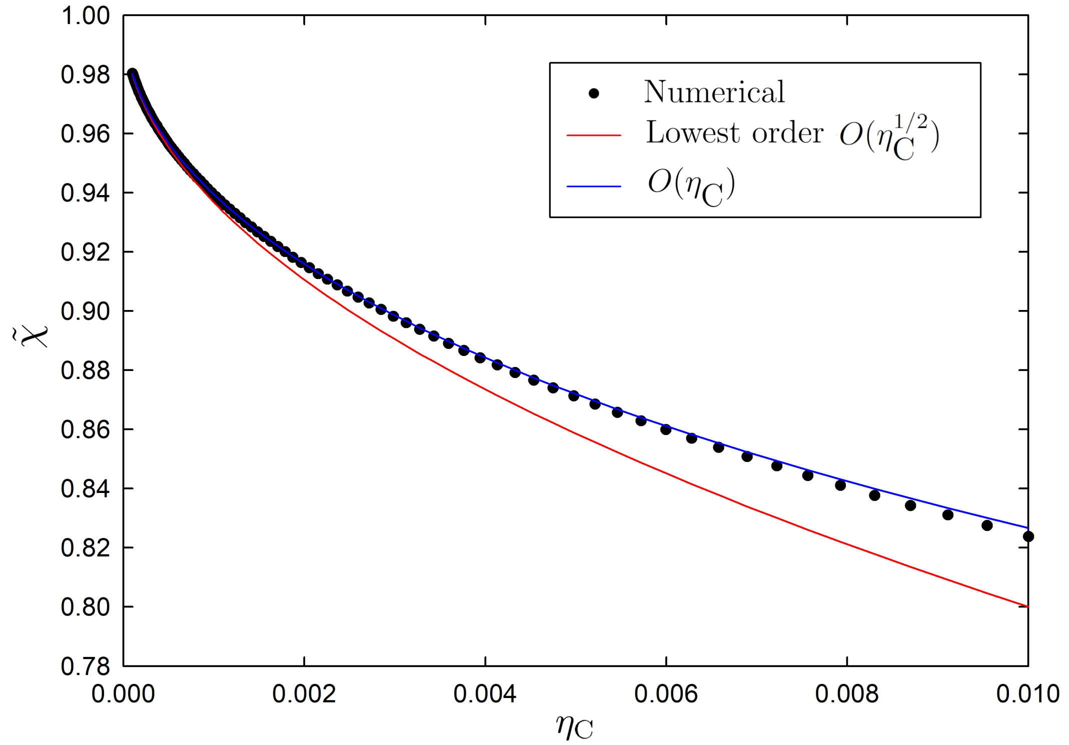


**Figure 7.** Comparison of the numerical evaluation of $\chi$ with its theoretical value. The optimal $\chi$ is plotted as a function of $\eta_C$. Numerics (circles) is compared with the theoretical estimate stemming from the series in equations (S31), up to order $\eta_C^{1/2}$ (red line) and $\eta_C$ (blue line). The latter curve reproduces the observed behaviour in the whole considered interval of $\eta_C$.

$$\tilde{\gamma} = \frac{1}{4} + \frac{3}{16}\eta_C + O(\eta_C^2), \tag{S32}$$

$$\tilde{\delta} = \frac{1}{4} - \frac{1}{4}\eta_C^{1/2} + \frac{19}{48}\eta_C - \frac{23}{72}\eta_C^{3/2} + O(\eta_C^2). \tag{S33}$$

Note that, introducing equation (S31) into equation (S19), we get the same results up to order $\eta_C^{1/2}$. Higher orders do not match due to the singular behaviour of the coefficients of our first expansion for fixed $\chi$ in the limit $\chi \to 1$, which produces an effective lowering of the orders in $\eta_C$. This reveals the need of the new expansion in this section to get a consistent result.

In Figure 7, we compare the numerically evaluated values of $\tilde{\chi}$ (circles) with the theoretical estimates given by the substitution of equation (S31) into equation (S26), up to order $\eta_C^{1/2}$ (red line) and $\eta_C$ (blue line). In the whole displayed range of $\eta_C$, we found an excellent agreement between the numerics and our theory.

Finally, we can get the optimal power and its corresponding efficiency by substitution of equations (S31)-(S33) in the expansion of $\widetilde{\mathcal{P}}$ and $\tilde{\eta}$ up to order $\eta_C^4$ and $\eta_C^3$, respectively, which yield the results given equations (46) and (47) of the main text. On a mathematical note, it should be stressed that $\widetilde{\mathcal{P}}$ and $\tilde{\eta}$ are not analytic functions of $\eta_C$. As a matter of fact, $\widetilde{\mathcal{P}}$ and $\tilde{\eta}$ are expanded in powers of $\eta_C^{1/2}$. Notwithstanding,

up to the considered order only $\widetilde{\mathcal{P}}$ contains non-integer powers of $\eta_{\mathrm{C}}$.

## References

[1] Bender C M and Orszag S A 1999 *Advanced mathematical methods for scientists and engineers I: Asymptotic methods and perturbation theory* (Springer)
[2] Schmiedl T and Seifert U 2008 *EPL (Europhysics Letters)* **81** 20003
[3] Esposito M, Lindenberg K and Broeck C V d 2009 *EPL (Europhysics Letters)* **85** 60010
